# Supplementary material for: Retrieval Augmented Generation and Understanding in Vision: A Survey and New Outlook
Source: arXiv:2503.18016 source file (2025-03-23)
Supplement: Supplementary file 1 [file appendix.tex]

\begin{table*}[t]
\caption{Comparison of Recent Video Understanding Benchmarks. This table presents a comprehensive overview of recent benchmarks categorized by their primary evaluation focus. The scale information is approximate and based on reported numbers in the papers. Some benchmarks may use multiple metrics or combined datasets.}
\label{tab:benchmarks}
\centering
\resizebox{\textwidth}{!}{

\begin{tabular}{llllll}
\toprule
Category & Benchmark & Year & Scale & Key Features & Evaluation Focus \\
\midrule
\multirow{5}{*}{\textbf{Fundamental}} & CG-Bench~\cite{Chen} & 2024 & 10K videos & Clue-grounded QA & Long video comprehension \\
Capabilities & OVO-Bench~\cite{li2025ovo} & 2025 & 5K videos & Online streaming & Real-time understanding \\
& Online Video Understanding~\cite{huang2024online} & 2024 & 8K videos & Continuous processing & Temporal awareness \\
& FIBER~\cite{xu2024fine} & 2024 & 1K videos & Fine-grained annotations & Spatial-temporal retrieval \\
& Reversed in Time~\cite{du2024reversed} & 2024 & 3K videos & Time-reversed negatives & Temporal reasoning \\
\midrule
\multirow{3}{*}{\textbf{Domain-specific}} & SCBench~\cite{ge2024scbench} & 2024 & 2K sports videos & Commentary generation & Sports understanding \\
& HumanVBench~\cite{zhou2024humanvbench} & 2024 & 17 task types & Human behavior analysis & Emotion \& interaction \\
& StoryEval~\cite{wang2024your} & 2024 & 1.5K narratives & Event sequence evaluation & Story comprehension \\
\midrule
\multirow{5}{*}{\textbf{Technical}} & Video OCR Study~\cite{fei2024current} & 2024 & Multiple datasets & OCR capability testing & Text recognition \\
Components & RAG-Check~\cite{mortaheb2025rag} & 2025 & Synthetic data & Hallucination detection & Generation reliability \\
& Frame Sampling Study~\cite{kandhare2024empirical} & 2024 & Comparative analysis & Sampling efficiency & Retrieval performance \\
& MMDocIR~\cite{dong2025mmdocir} & 2025 & 313 documents & Multi-level annotations & Document retrieval \\
\bottomrule
\end{tabular}
}
\end{table*}

\subsubsection{Benchmark Datasets for Video Understanding.}
The evolution of video understanding and retrieval systems has necessitated increasingly sophisticated evaluation frameworks to assess their real-world effectiveness. Recent benchmarks have emerged to address specific technical challenges while pushing the boundaries of comprehensive evaluation. We categorize and analyze these benchmarks based on their primary focus areas and technical contributions.
Fundamental capability assessment represents the first major direction in benchmark development. CG-Bench~\cite{Chen} pioneered clue-grounded question answering for long videos, addressing the critical challenge of information localization and utilization across extended sequences. This was complemented by OVO-Bench~\cite{li2025ovo} and the Online Video Understanding benchmark~\cite{huang2024online}, which specifically target temporal awareness and real-time processing capabilities - key requirements for streaming applications. Fine-grained comprehension evaluation has seen significant advances through FIBER~\cite{xu2024fine}, which introduces detailed spatial-temporal annotations, while Reversed in Time~\cite{du2024reversed} innovatively challenges temporal reasoning through carefully crafted negative samples. However, these benchmarks still struggle to fully capture the complexity of real-world scenarios, particularly in terms of multi-modal interaction and contextual understanding.
Domain-specific evaluation has emerged as another crucial direction, reflecting the increasing specialization of video understanding systems. SCBench~\cite{ge2024scbench} sets new standards for sports commentary generation, requiring both precise visual understanding and deep domain knowledge. HumanVBench~\cite{zhou2024humanvbench} advances human-centric analysis through comprehensive evaluation of emotion recognition and behavior interpretation. StoryEval~\cite{wang2024your} pushes the boundaries of narrative comprehension assessment. While these benchmarks provide valuable domain-specific insights, they highlight the ongoing challenge of balancing specialized evaluation with general-purpose applicability.
Technical component evaluation represents the third major direction, focusing on specific capabilities crucial for comprehensive video understanding. Fei et al.~\cite{fei2024current} specifically address OCR evaluation, highlighting a critical yet often overlooked aspect of information extraction. RAG-Check~\cite{mortaheb2025rag} introduces novel metrics for assessing hallucination in multi-modal RAG systems, while Kandhare et al.~\cite{kandhare2024empirical} provide empirical insights into sampling strategies. MMDocIR~\cite{dong2025mmdocir} extends evaluation to multi-modal document retrieval, incorporating both page-level and layout-level assessments. However, the field still lacks standardized metrics for comparing different technical approaches, particularly in terms of efficiency and scalability.
These diverse benchmarks collectively highlight both the progress and remaining challenges in video understanding evaluation. While current benchmarks effectively assess individual capabilities, the field still needs more comprehensive frameworks that can evaluate system-level performance across multiple dimensions simultaneously. Additionally, the rapid evolution of video understanding technologies necessitates continuous benchmark development to keep pace with emerging capabilities and applications.
